# Supplementary material for: Reinforcement Learning from Automatic Feedback for High-Quality Unit Test Generation
Source: arXiv:2310.02368 source file (2025-01-06)
Supplement: Supplementary file 2 [file 06-appendix.tex]

\appendix
